# Supplementary material for: A probabilistic latent variable model for detecting structure in binary data
Source: arXiv:2201.11108 source file (2022-01-26)
Supplement: Supplementary file 1 [file supp_CA.tex]

\section{Cell Assembly Model Supplement} \label{model_dev}

We reserve this supplemental text to catalog and give brief discussion on details of the Cell Assembly Model. This includes known issues and limitations, work thought about or begun but not followed through with, pointers to ideas to try in the future for anyone continuing with this, and other things not mentioned in the body of the paper.

\begin{enumerate}
    \item We focused our analysis on spike-words with 5ms binning because they yielded the most robust structure, although some structure was found in 3ms binned spike-words as well.
    
    \item For another comparison and a stronger model beyond the independent GLM, one should run pairwise GLM simulation for groups of cells ($\sim10-20$) that participate in particularly interesting looking CAs.
    
    \item The size of the latent dimension, $M$, is a hyper-parameter of the model. We did some initial investigation into over- and under-complete models with synthetic data, with $M>N$ and $M<N$ respectively. We hypothesize that model completeness will effect the type of structure discovered by CAs, especially when using the "Homeostatic Egalitarian" prior.
    
    \item When CAs in the same model are often co-active, do they provide redundant or synergistic information? Defined by:
    
    \begin{equation} \label{Synergy}
         S(a,b) = 1 - \sqrt{  cs_\tau(a,b) \cdot cs_M(a,b) }
    \end{equation}
    
    \noindent where $cs_\tau(a,b)$ and $cs_M(a,b)$ are the temporal and membership cosine similarity between CAs $a$ and $b$ within the same model. For a single CA, we are most interested in the minimum $S$ value across the rest of the population. Visualizing individual CAs does not reveal the full picture because observed spike words can be explained by simultaneous activity of multiple CAs. We look for CAs within a model that are commonly coactive, determined by cosine similarity of their PSTHs to determine if they have form interesting larger shapes. Fig.~\ref{coactive_offBT} shows CA (in red) along with two additional CAs with which it shares a large temporal overlap. Red and green CAs have more overlapping spatial and temporal representation in panel a and more synergistic representation in panel c. Panel b shows $z0$ example from above in red. Even this does not reveal the full picture. These CAs are determined to be temporally coactive by cosine similarity of PSTHs binned at 50ms. First, this does not indicate that they are necessarily coactive in the same trials. Second, if coactive in the same trials, they could at different times within the 50ms bins.
    
    \begin{figure}[H]
        \centering
        \begin{subfigure}{.25\textwidth}
            \includegraphics[width=\textwidth]{Figures_PGM/realData_section/offBT_Dont_Egal/coactiveRedundant_[offBriskTransient]_NatMov_5msBins_DontSmp1st_EgalQ_rand1B_z32.png}
            \caption{Redundant}
        \end{subfigure}
        \begin{subfigure}{.25\textwidth}
            \includegraphics[width=\textwidth]{Figures_PGM/realData_section/offBT_Dont_Egal/coactiveSynergy_[offBriskTransient]_NatMov_5msBins_DontSmp1st_EgalQ_rand2_z6.png}
            \caption{$z6$ example above}
        \end{subfigure}
        \begin{subfigure}{.25\textwidth}
            \includegraphics[width=\textwidth]{Figures_PGM/realData_section/offBT_Dont_Egal/coactiveSynergy_[offBriskTransient]_NatMov_5msBins_DontSmp1st_EgalQ_rand1B_z43.png}
            \caption{Synergistic}
        \end{subfigure}
        \caption{ \tiny{\textbf{ Coactive CAs can be synergystic or redundant:} \textit{ Bottom} PSTH traces show high temporal overlap between activations of 3 CAs. \textit{ Top left} shows high RF overlap for those CAs as well.} }
        \label{coactive_offBT}
    \end{figure}

    \noindent Empirically on the time-scale of individual spike-words, CAs are not often co-active relative to the number of times they are active individually. Fig.~\ref{coactive_matrix} shows a few typical, randomly sampled examples.
    
        \begin{figure}[H]
        \centering
        \begin{subfigure}{.4\textwidth}
            \includegraphics[width=\textwidth]{Figures_PGM/realData_section/CA_coactivity/[offBriskTransient]_NatMov_5msBins_DontSmp1st_EgalQ_rand0B.png}
            \caption{[offBT]}
        \end{subfigure}
        \begin{subfigure}{.4\textwidth}
            \includegraphics[width=\textwidth]{Figures_PGM/realData_section/CA_coactivity/[offBriskTransient,onBriskTransient]_NatMov_5msBins_DontSmp1st_BinomQ_rand0B.png}
            \caption{[offBT,onBT]}
        \end{subfigure}
        \caption{ \tiny{\textbf{CA individual inference and coactivity statistics:} Two panels show statistics for inference on all spike-words in data corpus after model is learned and fixed. Cell-type listed in panel caption. In each panel, CAs on x-axis. Blue points show number of time each CA was inferred across all spike-words. Red points show total number of times it was inferred with a partner. Top plot shows pairwise inference coactivity with 5 largest values circled in red. Coactivity among CAs is pretty insignificant.} }
        \label{coactive_matrix}
    \end{figure}

    \item We construct spike-words with a bin-size of 5ms but a step-size of 1ms. So individual spikes are used in multiple spike-words. This process introduces noisy repeats into spike words used introducing a couple of confounds. First, spike-words are used for learning and introduced noisy repeat structure can be confounded with structure in with actual noisy repeats from cell assemblies. Second, these spike-words are also used inference, to construct CA activity rasters. We attempted to do an ISI / Fano factor analysis to uncover periodic structure in CA activity, but had many 1ms and 2ms ISIs introduced by how the data set was constructed. 
        
    \item $\Delta$Py is an approximate, imperfect measure that introduces some confounds into the comparison with the GLM p(y). It correctly obtains high values when a CA is active and GLM rates predict low synchrony. However, large $\Delta$Py values (ie. small cosine similarity values) may also result from GLM predicted activity not observed in $z_a$'s PSTH. This may not reflect real significance because multiple CAs can learn overlapping cell membership and predicted activity at one moment can be partially or fully subsumed in the activity of another CA, leaving the first, $z_a$, inactive. However, $\Delta$Py only considers the PSTH of $z_a$, and the high activity at one time in $\langle p(\vec{y}_{null}) \rangle$ which is unmatched in the PSTH dramatically changes the angle between vectors in high dimensional space because it lowers the height or significance of other events in $\langle p(\vec{y}_{null}) \rangle$ relative to that max. This results in a low cosine similarity and a high significance in cases where similar CAs in the same model work together to to represent the activity of cells at different times. A more complete significance measure would consider the membership overlap of CAs in a model and allow for additional CAs with similar membership to absorb some of the GLM model prediction. It is probably not too hard to extend it to allow the significance comparison to use PSTHs from a couple $z_a$'s with very similar spatial/membership similarity. \label{delPy_caveats}
        
    \item An additional measure of the difference of spiking activity given $z_a=1$ from null model predictions is the KL-divergence between N-dimensional multivariate Bernoulli distributions of $p(y_i)_{null}$ and $p(y_i \vert z_a=1, z_{\not a}=0)$, shown and mentioned in Fig.~\ref{Del_Py_null}. It more explicitly makes the same confounding and faulty assumption that all other $z_{\not a}$'s are inactive. It may provide a more straight-forward path to generalize the $\Delta$Py metric. \label{KL_nDim_Bern}   
        
\end{enumerate}
